# Supplementary material for: CLIPLoss and Norm-Based Data Selection Methods for Multimodal Contrastive Learning
Source: arXiv:2405.19547 source file (2024-12-20)
Supplement: Supplementary file 1 [file experiment_appendix.tex]

\section{Details of Experiments}

\subsection{Training Configuration} \label{sub: config}
For the training sets, we choose ViT-B/32 model as the baseline, with training computations fixed at $9.5\times 10^{16}$ total multiply-accumulate operations (MACs), in line with the Datacomp~\cite{gadre2023datacomp} standards. All experiments were conducted on NVIDIA A40 GPUs.

% \subsection{Evaluation Datasets}\label{sub: eva datasets}
% We list all the evaluation sets here, and the details are in \citet{gadre2023datacomp}.
% \begin{itemize}
%     \item \textbf{ImageNet.} ImageNet-1k~\cite{deng2009imagenet}, 
%     \item \textbf{Visual Task Adaptation Benchmark (VTAB).}
%     \item \textbf{WILDS} 
%     \item \textbf{Retrieval.} Flickr30k~\cite{young-etal-2014-image}, MSCOCO~\cite{chen2015microsoft} and WinoGAViL~\cite{bitton2022winogavil}.
% \end{itemize}

% We evaluate our model on 38 datasets related to image classification and retrieval tasks adopted in DataComp. The image classification tasks 
% vary from visual recognition to distance prediction, 
% contain , ImageNet distribution shifts~\cite{wang2019learning,pmlr-v97-recht19a,hendrycks2021natural,hendrycks2021many}, 11 datasets from the Visual Task Adaptation Benchmark (VTAB)~\cite{zhai2019large} and 3 datasets from  ~\cite{koh2021wilds, sagawa2021extending}, which tests the robustness facing subpopulation shift and spurious correlation. Retrieval datasets contain  which focus on image-text retrieval and  related to commonsense association.
\subsection{Baselines}\label{sub: baselines}
We add some details about the baselines used in our paper.
\begin{itemize}[leftmargin=*]
    \item \textbf{Text-based filtering.}  \citet{gadre2023datacomp} proposes a text-based filtering that tries to select the data that contains caption overlapping with the class name from ImageNet-21K or ImageNet-1K. We just apply this filter on DataComp because this heuristic method cannot determine the size of the selected pool of data, and thus not suitable for the coreset selection scenario on CC12M.
    \item \textbf{Image-based filtering.}  \citet{gadre2023datacomp} also proposes a heuristic way to sample the visual content overlaps with ImageNet-1K classes. They first apply filtering by language (only choose English caption by fasttext~\cite{joulin2016bag}) and caption length (over two words and 5 characters). Then they cluster the image embeddings from training data to 100K groups using Faiss~\cite{johnson2019billion}, and keep the groups whose cluster center is the nearest neighbor to at least one image embedding of ImageNet-1K image. 
    \item \textbf{$\mathbb{D}^2$ Pruning.}  \citet{maharana2023d2} tries to represent the dataset as an undirected graph for coreset selection. They assign the difficulty for each example and use message passing to update the difficulty score incorporating the difficulty of its neighboring examples, and finally try to keep both diverse and difficult subsets. For our experiments, we adhere to the default hyperparameters of $\mathbb{D}^2$ on DataComp as specified in their official codebase. Additionally, we tune the number of nearest neighbors over $k = \{1,5,10,15\}$ and report their best results on CC12M, following their recommendations in the paper.
\end{itemize}
\subsection{Algorithm Details}\label{sub: algo details}
In this section, we illustrate the details of our VAS-D algorithm, the generation of text embeddings of ImageNet-1k, and the choice of hyperparameters.

\paragraph{VAS-D.} We use greedy remove methods to achieve the object (\ref{eq:tr_S2}). Note that if the number of greedy steps is $\tau$, and let $\bar\Sigma_{\text{test},i} = \frac{1}{|S_i|}\sum_{j \in S_i}\bar f_v(\vx_j^v)\bar f_v(\vx_j^v)^\top$ where $S_i$ is the selected subset at step $i$, then obtaining (\ref{eq:tr_S2}) with step-by-step greedy remove is equivalent to removing the data satisfies (\ref{eq:greedy}):
\begin{equation}\label{eq:greedy}
    S_{i} \setminus S_{i+1} = \arg \max_{p \in S_{i}} \Tr\left((\bar \Sigma_{\text{test},i} - f_v(\vx_p^v)\bar f_v(\vx_p^v)^\top)^2\right) = \arg \min_{p \in S_{i}} \left[\bar f_v(\vx_p^v)^T \cdot\bar \Sigma_{\text{test},i}\cdot\bar f_v(\vx_p^v)\right], \quad i \in \{0, \ldots, \tau-1\}
\end{equation}
Then we can detail the algorithm process of VAS-D in Algorithm~\ref{algo: VAS-D}. In experiments, we all fix the number of greedy step $\tau$ to $168$ on both DataComp and CC12M. But this is not a parameter that needs to be finely tuned. Generally, the selected subset is well when $\tau > 100$ for DataComp and CC12M. 

\begin{algorithm}
\caption{VAS-D with greedy remove strategy}
\label{algo: VAS-D}
\begin{algorithmic}
    \STATE {\bfseries Inputs:} image embeddings of the data after CLIP score filtering $\{\bar f_v(\vx_i^v)\}_{i \in S}$, target size $N$, number of greedy steps $\tau$
    \STATE Initialize $S_0 = S, N_0 = |S|$
    \FOR{$t=1$ {\bfseries to} $\tau$}
    \STATE Size at step $t$ : $N_t = N_0 - \frac{t}{\tau}(N_0 - N)$.
    \STATE Prior matrix: $\bar\Sigma_{\text{test}, t-1} = \sum_{j \in S_{t-1}}\bar f_v(\vx_j^v)\bar f_v(\vx_j^v)^\top$
    \STATE Updated VAS for each sample $p$ in $S_{t-1}$: $\text{VAS}_p = \bar f_v(\vx_p^v)^\top\cdot \bar\Sigma_{\text{test}, t-1}\cdot \bar f_v(\vx_p^v)$
    \STATE Construct $S_t$ such that it contains the data with highest VAS in $S_{t-1}$ and satisfies $|S_t| = N_t$. 
    \ENDFOR
    % \STATE \textbf{Step 1:} \textit{Conservatively} remove low CLIP score samples. (i.e., almost certain low-quality samples)
    % \STATE \textbf{Step 2.1:} Choose proper $\vD_{\text{test\_proxy}}$
    % \STATE \textbf{Step 2.2:} Select $S = \arg \max_{|S| = N} \sum_{i \in S}\text{VAS}_i(v,v)$
\end{algorithmic}
\end{algorithm}

% \begin{algorithm}[tb]
%    \caption{Bubble Sort}
%    \label{alg:example}
% \begin{algorithmic}
%    \STATE {\bfseries Input:} data $x_i$, size $m$
%    % \REPEAT
%    \STATE Initialize $noChange = true$.
%    \FOR{$i=1$ {\bfseries to} $m-1$}
%    \IF{$x_i > x_{i+1}$}
%    \STATE Swap $x_i$ and $x_{i+1}$
%    \STATE $noChange = false$
%    \ENDIF
%    \ENDFOR
%    % \UNTIL{$noChange$ is $true$}
% \end{algorithmic}
% \end{algorithm}

\paragraph{Text embeddings of ImageNet-1k.}
In the ablation study (Tab.~\ref{tab:abla}), we use text embedding from ImageNet-1k to calculate VAS. There we select 80 templates as \cite{radford2021learning} for prompt generation for each class and take the mean of their embeddings as the representative text embedding for images within that class. 

\subsection{Hyperparameters}\label{sub: hyperp}
% The main hyperparameters of our algorithm (Alg.~\ref{algo: main} and Alg.~\ref{algo: VAS-D}) are the target number of CLIP score filtering and VAS filtering. In this paper, we just fix the size of the final pool to be 30\% of the original dataset and restrict CLIP score filtering to get around 50\% of data from the original pool.

% However, a better way to choose these two hyperparameters is to \textbf{choose the filtering threshold for CLIP score and VAS filtering}. The reason is that when the teacher model is fixed, and the test prior is chosen to be ImageNet-1k, then both the CLIP score and VAS score are just relevant to each sample itself and not to the rest of the data, which means that the threshold should be \textbf{training-dataset-independent}. So we should be able to transfer the threshold to different datasets. For our experiment on DataComp, the thresholds for CLIP score and VAS are roughly \textbf{0.214} and \textbf{0.153}, respectively, and we recommend other researchers to try the initial threshold at around these values when execuating our algorithm. 

The main hyper-parameters of our algorithm (Alg.~\ref{algo: main} and Alg.~\ref{algo: VAS-D}) are the target numbers after CLIP score filtering and VAS filtering. In this paper, we choose CLIP score filtering to get around 50\% of data from the original pool and the VAS filtering to further get 30\% of data from the original pool . This is approximately equivalent to setting CLIP score threshold as \textbf{0.214} and VAS threshold as \textbf{0.153}. 
To give readers a more intuitive understanding of how these two thresholds select most of the high-quality and informative data, we provide a visualization with different CLIP scores and VAS scores in Fig.~\ref{fig:vis_many}.

Notably, the choice of both thresholds is \textbf{train-dataset-independent}. That is, the CLIP score only evaluates individual data quality without considering the whole train data distribution;  Similarly, VAS, according to our definition, is only dependent on individual data embedding and the test prior (ImageNet-1k in our case). Such independence suggests that, when the teacher embedding model and the test prior is fixed, our threshold choice can be potentially transferred to other train datasets. So we recommend other researchers to try the initial threshold at around these values when executing our algorithm.

In addition, for VAS-D where the test-prior is highly related to the training dataset, there also exists an easy way to decouple. Specifically, we can use VAS(ImageNet-1k) as data prior to estimate the target number after VAS-D filtering and then apply VAS-D(Traindata) as Alg.~\ref{algo: VAS-D}. In this way, our methods can also be used with little or no parameter tuning.

\subsection{Time Cost}\label{sub: time cost}
We compare the time cost for different methods on 1 NVIDIA A40 GPU in Tab.~\ref{tab:time}. Here since all the key approaches in this paper require obtaining embeddings, so we don't take the time of calculating image/text embeddings with the pretrained CLIP model into consideration. We can observe that our VAS(ImageNet-1k/Dataset) + CLIP score filtering is extremely time efficient. Although VAS-D takes longer time due to the multi-step greedy removal process, it's acceptable compared with total training time and still faster than image-based filtering which requires Faiss~\cite{johnson2019billion} for clustering. 
% \yifang{I think VAS-D and Image-based approch does not have significant difference, also this go back to the problem that comparing to training time, those are all not dominant time cost... So I am not sure if we should highlight this in main paper. }\yiping{Can be put into appendix}
\begin{table}
\small
\centering
\caption{Approximate time cost for different methods on DataComp with 1 NVIDIA A40.}
\label{tab:time}
\begin{tabular}{@{}lc@{}}
\toprule
  & Time Cost\\ \midrule
CLIP Score  & $<$\textbf{1m}\\
Image-based & 1h\\
$\mathbb{D}^2$ Pruning & 25m\\
VAS(ImageNet-1k/DataComp) & $<$\textbf{1m}\\
VAS-D(DataComp) &  36m\\
\midrule
Training Time & 16h\\
\bottomrule
\end{tabular}
\end{table}

\newpage
\section{Ablation Study on CLIPLoss}

\begin{table*}[ht]
\small
\centering
\vspace{-1em}
\caption{Results of CLIPLoss with different number of batch sampling (denoted as `sn') on DataComp-medium. All the methods use OpenAI's CLIP-L/14 as the pretrained model. }
\vspace{0.3em}
\label{tab:CLIPLpss_batch_num}
\begin{tabular}{@{}lcccccc@{}}
\toprule
\multirow{2}{*}{
\textbf{Filtering Strategy}} & \textbf{Dataset} & \textbf{IN-1k} & \textbf{IN Dist. Shift} & \textbf{VTAB} & \textbf{Retrieval} & \textbf{Average} \\
 & \textbf{Size} & (1 sub-task) & (5) & (11) & (3) & (38)\\
 \midrule
 CLIPScore (20\%) & 22M & 25.4 & 22.7 & 31.8 & 22.0 & 31.0 \\
CLIPLoss (20\%, sn=1) & 22M & 26.7 & 23.1 & 31.9 & 23.0 & 31.1\\
CLIPLoss (20\%, sn=5) & 22M & 27.3 & 23.8 & 34.1 & \textbf{24.1} & \textbf{32.7}\\
CLIPLoss (20\%, sn=10) & 22M & 27.4 & 23.8 & 33.7 & 23.7 & 32.5\\
CLIPLoss (20\%, sn=20) & 22M & {27.5} & 24.0 & 32.8 & 23.2 & 32.4\\
CLIPLoss (20\%, sn=50) & 22M & \textbf{27.7} & \textbf{24.1} & \textbf{34.3} & 23.7 & 32.6\\
CLIPLoss (20\%, sn=100) & 22M & {27.1} & {23.9} & {34.0} & 24.3 & 32.3\\
\midrule
CLIPScore (30\%) & 33M & 26.4 & 23.6 & 32.6 & 24.5 & 32.2 \\
CLIPLoss (30\%, sn=1) & 33M & 27.6& 24.1& 33.7& \textbf{25.3}& 32.7\\
CLIPLoss (30\%, sn=5) & 33M & \textbf{28.1} & \textbf{24.7} & 32.7 & 24.9 & 32.6\\
CLIPLoss (30\%, sn=10) & 33M & 27.9 & 24.6 & 33.2 & 25.1 & \textbf{32.9}\\
CLIPLoss (30\%, sn=50) & 33M & 28.0 & 24.3 & \textbf{34.5} & 24.8 & 32.8\\

% No filtering  & 12.8M & 2.5 & 3.3 & 14.5 & 10.5 & 13.2 \\
% Text-based filtering  & 3.2M & 4.6 & 5.2 & 16.9 & 11.2 & 15.6 \\
% Image-based filtering  & 3.0M & 4.3 & 4.7 & 17.8 & 11.2 & 15.8 \\
% % \rowcolor[HTML]{EFEFEF} 
% CLIP score (30\%)  & 3.8M & {5.1} & {5.5} & 19.0 & 10.8 & 17.2 \\
% $\mathbb{D}^2$ Pruning (image+text)  & 3.8M & {5.1} & {5.6} & {18.2} & {11.7} & 17.0 \\
% Image-based $\cap$ CLIP score (30\%) & 1.4M& 3.9& 4.5& 16.2& 8.9 & 14.4\\
% % Image-based filtering \cite{gadre2023datacomp} (reproduced) & 3.0M & 4.1 & 4.6 & 17.5 & 11.6 & 15.7 \\
% \midrule
% CLIP score (30\%, reproduced) & 3.8M & {4.8} & 5.3 & 17.1 & 11.5 & 15.8 \\
% Image-based $\cap$ CLIP score (45\%)  & 1.9M & 4.2 & 4.6& 17.4& 10.8 & 15.5 \\
% $\mathbb{D}^2$ Pruning (image+text, reproduced) & 3.8M & 4.6 & 5.2 & {18.5} & 11.1 & 16.1 \\
% CLIP score (45\%) & 5.8M & 4.5 & 5.1 & 17.9 & \textbf{12.3} & 16.1 \\
% \midrule
% \textbf{VAS} (ImageNet-1k) %\yiping{Need place this here?}
% & 3.8M & 2.4& 3.1& 14.9& 10.4& 12.7 \\
% \textbf{VAS} (ImageNet-1k) $\cap$ 
% CLIP score 
% (45\%) 
% & 3.8M & \textbf{5.2} & \textbf{5.5} & \underline{19.0} & \underline{12.2} & \textbf{17.4} \\
% % \textbf{VAS} (DataComp) & 3.8M & & & & & \\
% \textbf{VAS} (DataComp) $\cap$ CLIP score 
% (45\%)
% & 3.8M & \underline{5.0} & \underline{5.4} & 17.9 & {12.1} & 16.2\\
% % \textbf{VAS-D} (DataComp) & 3.8M & & & & & \\
% \textbf{VAS-D} (DataComp) $\cap$ CLIP score 
% (45\%) 
% & 3.8M & 4.7 & \underline{5.4} & \textbf{19.7} & {11.7} & \underline{17.3} \\
\bottomrule
% \textsuperscript{D}2 PRUNING (image only) & 3.8M & 4.4 & 5.1 & 16.9 & 12.1 & 15.9 \\
% \textsuperscript{D}2 PRUNING (text only) & 3.8M & 4.9 & 5.5 & 17.0 & 12.3 & 16.6 \\ \bottomrule
\end{tabular}
\vspace{-1em}
\end{table*}

In the main paper, we assume `sn=10' for all the CLIPLoss-based experiments.

\begin{table*}[ht]
\small
\centering
\vspace{-1em}
\caption{Comparison between CLIPScore and CLIPLoss under different downsampling ratio. All the methods use OpenAI's CLIP-L/14 as the pretrained model. }
\vspace{0.3em}
\label{tab:CLIPLpss_batch_num}
\begin{tabular}{@{}lcccccc@{}}
\toprule
\multirow{2}{*}{
\textbf{Filtering Strategy}} & \textbf{Dataset} & \textbf{IN-1k} & \textbf{IN Dist. Shift} & \textbf{VTAB} & \textbf{Retrieval} & \textbf{Average} \\
 & \textbf{Size} & (1 sub-task) & (5) & (11) & (3) & (38)\\
\midrule
CLIPScore (1\%) & 1M & 1.3 & 2.0 & 15.6 & 6.4 & 10.9\\
CLIPLoss (1\%) & 1M & & & & & \\
 \midrule
CLIPScore (10\%) & 11M & 18.2 & 17.5 & 28.2 & 18.0 & 26.2\\
CLIPLoss (10\%) & 11M & 20.3 & 18.0 & 28.0 & 18.6 & 27.0\\
 \midrule
 CLIPScore (20\%) & 22M & 25.4 & 22.7 & 31.8 & 22.0 & 31.0 \\
CLIPLoss (20\%) & 22M & 27.4 & 23.8 & 33.7 & 23.7 & 32.5\\
\midrule
CLIPScore (30\%) & 33M & 26.4 & 23.6 & 32.6 & 24.5 & 32.2 \\
CLIPLoss (30\%) & 33M & 27.9 & 24.6 & 33.2 & 25.1 & {32.9}\\
\midrule
CLIPScore (40\%) & 44M & 26.1 & 22.9 & 32.4 & 25.4 & 31.9\\
CLIPLoss (40\%) & 44M & 26.8 & 23.4 & 31.9 & 25.0 & 32.2\\
 \midrule
CLIPScore (50\%) &  & 25.1& 22.1 & 29.8 & 24.9 & 30.8 \\
CLIPLoss (50\%) &  & & & & & \\
\midrule
CLIPScore (90\%) &   & 18.4 & 16.1 & 25.5 & 22.7 & 26.1\\
CLIPLoss (90\%) &  &  & & & & \\
\bottomrule
\end{tabular}
\vspace{-1em}
\end{table*}

\section{New Results}
\begin{table*}[ht]
\small
\centering
\vspace{-1em}
\caption{Results on DataComp-medium from methods that use only OpenAI's CLIP model. 
The `dataset size' is the size of the subset, which is obtained from different methods, of the whole training pool we could download.
% Method1 ($\alpha\%$) $\cap$ Method2 ($\beta\%$) denotes first use Method1 to filter to $\alpha\%$, then use Method 2 to filter to $\beta\%$ with respect to the original whole pool.
}
\vspace{0.3em}
\label{tab:OAI_only_result}
\begin{tabular}{@{}lcccccc@{}}
\toprule
\multirow{2}{*}{
\textbf{Filtering Strategy}} & \textbf{Dataset} & \textbf{IN-1k} & \textbf{IN Dist. Shift} & \textbf{VTAB} & \textbf{Retrieval} & \textbf{Average} \\
 & \textbf{Size} & (1 sub-task) & (5) & (11) & (3) & (38)\\
 \midrule
No filtering & 110M & 17.3 & 15.0 & 25.2 & 21.3 & 25.6 \\
% Text-based\footnote{Text-based filtering use fasttext~\citet{joulin2016bag} to select English captions.}
% & 26M & 24.8 & 22.2 & 30.1 & 24.2 & 29.5 \\
Image-based & 24M & 25.5 & 21.9 & 30.4 & 24.6 & 29.9 \\
CLIPScore (20\%) & 22M & 25.4 & 22.7 & 31.8 & 22.0 & 31.0 \\
CLIPScore (30\%) & 33M & 26.4 & 23.6 & 32.6 & 24.5 & 32.2 \\
Image-based $\cap$ CLIP score (30\%) & 11M & 27.4 & 23.9 & 31.9 & 21.4 & 30.8\\
\midrule
CLIPScore (30\%) $\cap$ $\text{VAS}_{2}$-D & 22M & {28.3} & {25.0} & {34.5} & {22.7} & {32.9}\\
CLIPScore (30\%) $\cap$ $\text{VAS}_{\infty}$-D & & & & & & \\
CLIPLoss (30\%) $\cap$ $\text{VAS}_{2}$-D & & & & & & \\
CLIPLoss (30\%) $\cap$ $\text{VAS}_{\infty}$-D & & & & & & \\
\midrule
CLIPScore (30\%) $\cap$ $\text{VAS}_{2}$(IN-1k) & 22M & {29.1} & {25.4} & \underline{35.8} & {24.1} & {33.4}\\
CLIPScore (30\%) $\cap$ $\text{VAS}_{2}$(Target) & 22M & 28.9 & 25.1 & 32.7 & 23.6 & 32.5\\
CLIPScore (30\%) $\cap$ $\text{VAS}_{\infty}$(IN-1k) & 22M & {29.7} & {25.9} & {33.7} & {24.1} & {33.7}\\
CLIPScore (30\%) $\cap$ $\text{VAS}_{\infty}$(Target) & 22M & 30.2 & 26.2 & 35.0 & 23.4& 33.9 \\
\midrule
CLIPLoss (20\%) & 22M & 27.4 & 23.8 & 33.7 & 23.7 & 32.5\\
CLIPLoss (30\%) & 33M & 27.9 & 24.6 & 33.2 & 25.1 & {32.9}\\
\midrule
CLIPLoss (30\%) $\cap$ $\text{VAS}_{2}$(IN-1k) & 22M & {30.4} & {26.4} & {35.4} & \underline{25.6} & {34.3}\\
CLIPLoss (30\%) $\cap$ $\text{VAS}_{2}$(Target) & 22M & 30.6 & 26.2 & 35.2 & 25.5 & 33.9 \\
CLIPLoss (30\%) $\cap$ $\text{VAS}_{\infty}$(IN-1k) & 22M & \textbf{31.9 }& \textbf{27.3} & 34.8 & 25.0 & \underline{34.4} \\
CLIPLoss (30\%) $\cap$ $\text{VAS}_{\infty}$(Target) & 22M & \underline{31.7} & \underline{27.2} & \textbf{36.0} & \textbf{26.0} & \textbf{35.0}\\
\bottomrule
\end{tabular}
\vspace{-1em}
\end{table*}

\begin{table*}[ht]
\small
\centering
\vspace{-1em}
\caption{Results on DataComp-medium from methods that need to use or train other models. 
The `dataset size' is the size of the subset, which is obtained from different methods, of the whole training pool we could download. Here all the baselines except MLM are reproduced. \yiping{If we need to add MLM?} DFN-P denotes the public version of the Data filtering network. `*' denotes the experiments reproduced using their official UIDs of the selected data, and `[XXX]' denotes the method using XXX as the pre-trained CLIP model, and the default model is OpenAI's CLIP-L/14.
% Method1 ($\alpha\%$) $\cap$ Method2 ($\beta\%$) denotes first use Method1 to filter to $\alpha\%$, then use Method 2 to filter to $\beta\%$ with respect to the original whole pool.
}
\vspace{0.3em}
\label{tab:OAI_only_result}
\begin{tabular}{@{}lcccccc@{}}
\toprule
\multirow{2}{*}{
\textbf{Filtering Strategy}} & \textbf{Dataset} & \textbf{IN-1k} & \textbf{IN Dist. Shift} & \textbf{VTAB} & \textbf{Retrieval} & \textbf{Average} \\
 & \textbf{Size} & (1 sub-task) & (5) & (11) & (3) & (38)\\
 \midrule
Text-based~\cite{gadre2023datacomp} & 26M & 24.8 & 22.2 & 30.1 & 24.2 & 29.5 \\
$\mathbb{D}^2$ Pruning~\cite{maharana2023d2} & 22M & 23.2 & 20.4 & 31.4 & 18.7 & 29.5\\
T-MARS*~\cite{maini2023t} & 22M & 30.8 & 26.3 & 34.8 & 25.4 & 34.1 \\
MLM~\cite{wang2024finetuned} & 38M & 30.3 & 25.6 & 36.0 & 29.0 & 34.5\\

Devil*~\cite{yu2023devil} & 20M & 31.0 & 26.7& 35.9 & 24.7 & 34.5\\
DFN*~\cite{fang2023data} & 16M & 36.0 & 30.1 & 36.2 & 27.0 & 35.4\\
DFN-P~\cite{fang2023data} & & & & & & \\
\midrule
DFN* $\cup$ \{CLIPLoss (20\%) $\cap$ $\text{VAS}_{\infty}$(Target) (10\%)\}\\
\yiping{need rerun and double check} 
% & & & & & & \\
& 21M & 34.3 & 29.5 & 38.2 & 27.1 & 36.2 \\
Devil* $\cup$ \{CLIPLoss (20\%) $\cap$ $\text{VAS}_{\infty}$(Target) (10\%)\} & & & & & & \\
\midrule
$\text{CLIPLoss}$ (30\%) $\cap$ $\text{VAS}_{2}$(IN-1k) [DFN-P] & & & & & & \\
$\text{CLIPLoss}$ (30\%) $\cap$ $\text{VAS}_{2}$(Target) [DFN-P] & & & & & & \\
$\text{CLIPLoss}$ (30\%) $\cap$ $\text{VAS}_{\infty}$(IN-1k) [DFN-P] & & & & & & \\
$\text{CLIPLoss}$ (30\%) $\cap$ $\text{VAS}_{\infty}$(Target) [DFN-P] & & & & & & \\
\bottomrule
\end{tabular}
\vspace{-1em}
\end{table*}

\newpage
\section{Data Pre-Processing Time}

% \begin{table*}[ht]
% \small
% \centering
% \vspace{-1em}
% \caption{Preprocessing model required by different methods and their estimated data pre-processing time (time unit is A40 hour) on DataComp-Medium, where we downloaded 111M data. Here since all the excellent baselines below use a pretrained CLIP model, we assume that the image/text CLIP embeddings have been obtained, which is also the case in DataComp benchmark~\citep{gadre2023datacomp}.}
% \vspace{0.3em}
% \label{tab:preprocess}
% \begin{tabular}{@{}lcccccc@{}}
% \toprule
% % \multirow{2}{*}{
% % \textbf{Filtering Strategy}} & Use CLIP model? & Other model used & Preprocess time & \textbf{Average acc} \\
% %  &  & (1 sub-task) & (5) & (11) & (3) & (38)\\
% %  \midrule

% \textbf{Filtering Strategy} & Other Model Used & Need to train that model? & Preprocess Time & \textbf{Average acc} \\
% \midrule
% T-MARS*~\cite{maini2023t} & Text Detection model~\cite{chen2021fast} & $\times$ & 950 h & 34.1\\
% MLM~\cite{wang2024finetuned} & LLaVA-1.5& $\surd$ & 1130 h & 34.5\\
% \bottomrule
% \end{tabular}
% \vspace{-1em}
% \end{table*}

Need to claim that our method is totally orthogonal to Data Filtering Network.

\begin{table*}[ht]
\centering
\small
\vspace{-1em}
\caption{Preprocessing model required by different methods and their estimated data pre-processing time (time unit is L40 hour) on DataComp-Medium, where we downloaded 111M data. Here since all the baselines below except MLM use a pretrained CLIP model, 
% we assume that the image/text CLIP embeddings have been obtained
we only count the time that doesn't contain that for infering CLIP image/text embeddings, which is also adopted in DataComp benchmark~\citep{gadre2023datacomp}. 
\yiping{Give out the time for using CLIP-B/32}}
\vspace{0.3em}
\label{tab:preprocess}
\begin{tabular}{@{}lccccc@{}}
\toprule
% \multirow{2}{*}{
% \textbf{Filtering Strategy}} & Use CLIP model? & Other model used & Preprocess time & \textbf{Average acc} \\
%  &  & (1 sub-task) & (5) & (11) & (3) & (38)\\
\multirow{2}{*}{\textbf{Filtering Strategy}} & \textbf{Other Model} & \textbf{Need (re-)train } & \textbf{Preprocess} & \textbf{Training} & \textbf{Average} \\
& \textbf{Used} & \textbf{that model?} & \textbf{Time} & \textbf{Time} & \textbf{acc}\\
\toprule
\multirow{2}{*}{{$\mathbb{D}^2$ Pruning}\cite{maharana2023d2}} & Graph\yiping{Need double check} & \multirow{2}{*}{$\surd$} & 
% \multirow{2}{*}{9 h} 
\multirow{2}{*}{70 h} 
& \multirow{2}{*}{65 h} & \multirow{2}{*}{29.5} \\
& \yiping{Need double check} & & & & \\
% \midrule
\multirow{2}{*}{{T-MARS} \cite{maini2023t}} & Text Detection Model: FAST & \multirow{2}{*}{$\times$} & \multirow{2}{*}{950 h} & \multirow{2}{*}{65 h} & \multirow{2}{*}{34.1} \\
& \cite{chen2021fast} & & & & \\
% \midrule
\multirow{2}{*}{{MLM} \cite{wang2024finetuned}} & Multimodal Language Model: LLaVA-1.5 & \multirow{2}{*}{$\surd$} & \multirow{2}{*}{1130 h} & \multirow{2}{*}{65 h} & \multirow{2}{*}{34.5} \\
& \cite{liu2023improved,chiang2023vicuna} & & & & \\
% \midrule
\multirow{2}{*}{{Devil} \cite{yu2023devil}} & PoS, fasttext, BLIP2  & \multirow{2}{*}{$\times$} & \multirow{2}{*}{} & \multirow{2}{*}{65 h} & \multirow{2}{*}{34.5} \\
& XXX & & & & \\
\toprule
CLIPLoss $\cap$ $\text{VAS}_{2}$(IN-1k) \textbf{(Ours)}
& NA & NA & 5 h & 65 h & 34.3 \\
% \midrule
CLIPLoss $\cap$ $\text{VAS}_{\infty}$(Target) \textbf{(Ours)} & NA & NA & \textbf{5 h} & 65 h & \textbf{35.0} \\
\bottomrule
\end{tabular}
\vspace{-1em}
\end{table*}

% Citation: 
% T-MAR

\newpage
\section{Additional Visualization}\label{sec: add_vis}
We further visualize more data with different CLIP scores and VAS in Fig.~\ref{fig:visual} and Fig.~\ref{fig:vis_many}. In Fig.~\ref{fig:vis_many} we can see that VAS(ImageNet-1k) always have similar score as VAS(DataComp).

Furthermore, we randomly sample 5000 data points from DataComp and calculate their CLIP score and VAS and scatter them in Fig.~\ref{fig:scatter}, we can see that after filtering out the data with top 50\% CLIP score, data with lower VAS may have higher probability for achieving high CLIP score, and data with higher VAS generally have a more centralized CLIP score range.

\begin{figure*}[h]
\centering
    \caption{Data distribution on VAS and CLIP score. We randomly sample 5000 points in DataComp and show its corresponding VAS and CLIP score, here VAS is calculated by the image embeddings from ImageNet-1k.}
    \includegraphics[width=0.5 \textwidth]{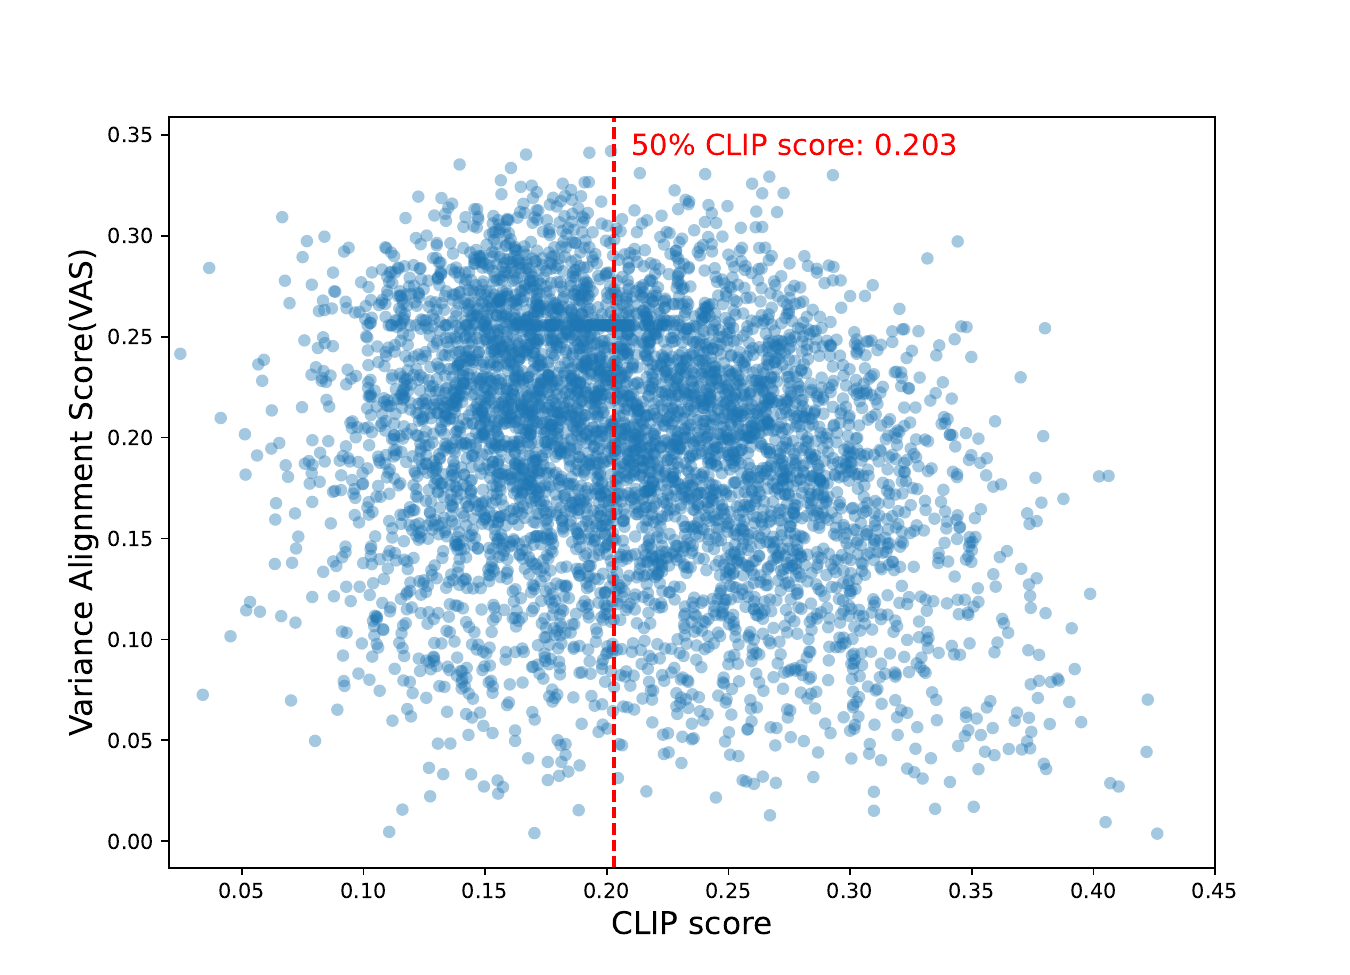}
    \label{fig:scatter}
    \vspace{-1em}
\end{figure*}

\begin{figure*}[h]
\centering
    % \vspace{-1em}
    \caption{Visualization of image data with different CLIP scores and VAS in DataComp.}
    \includegraphics[width=0.80 \textwidth]{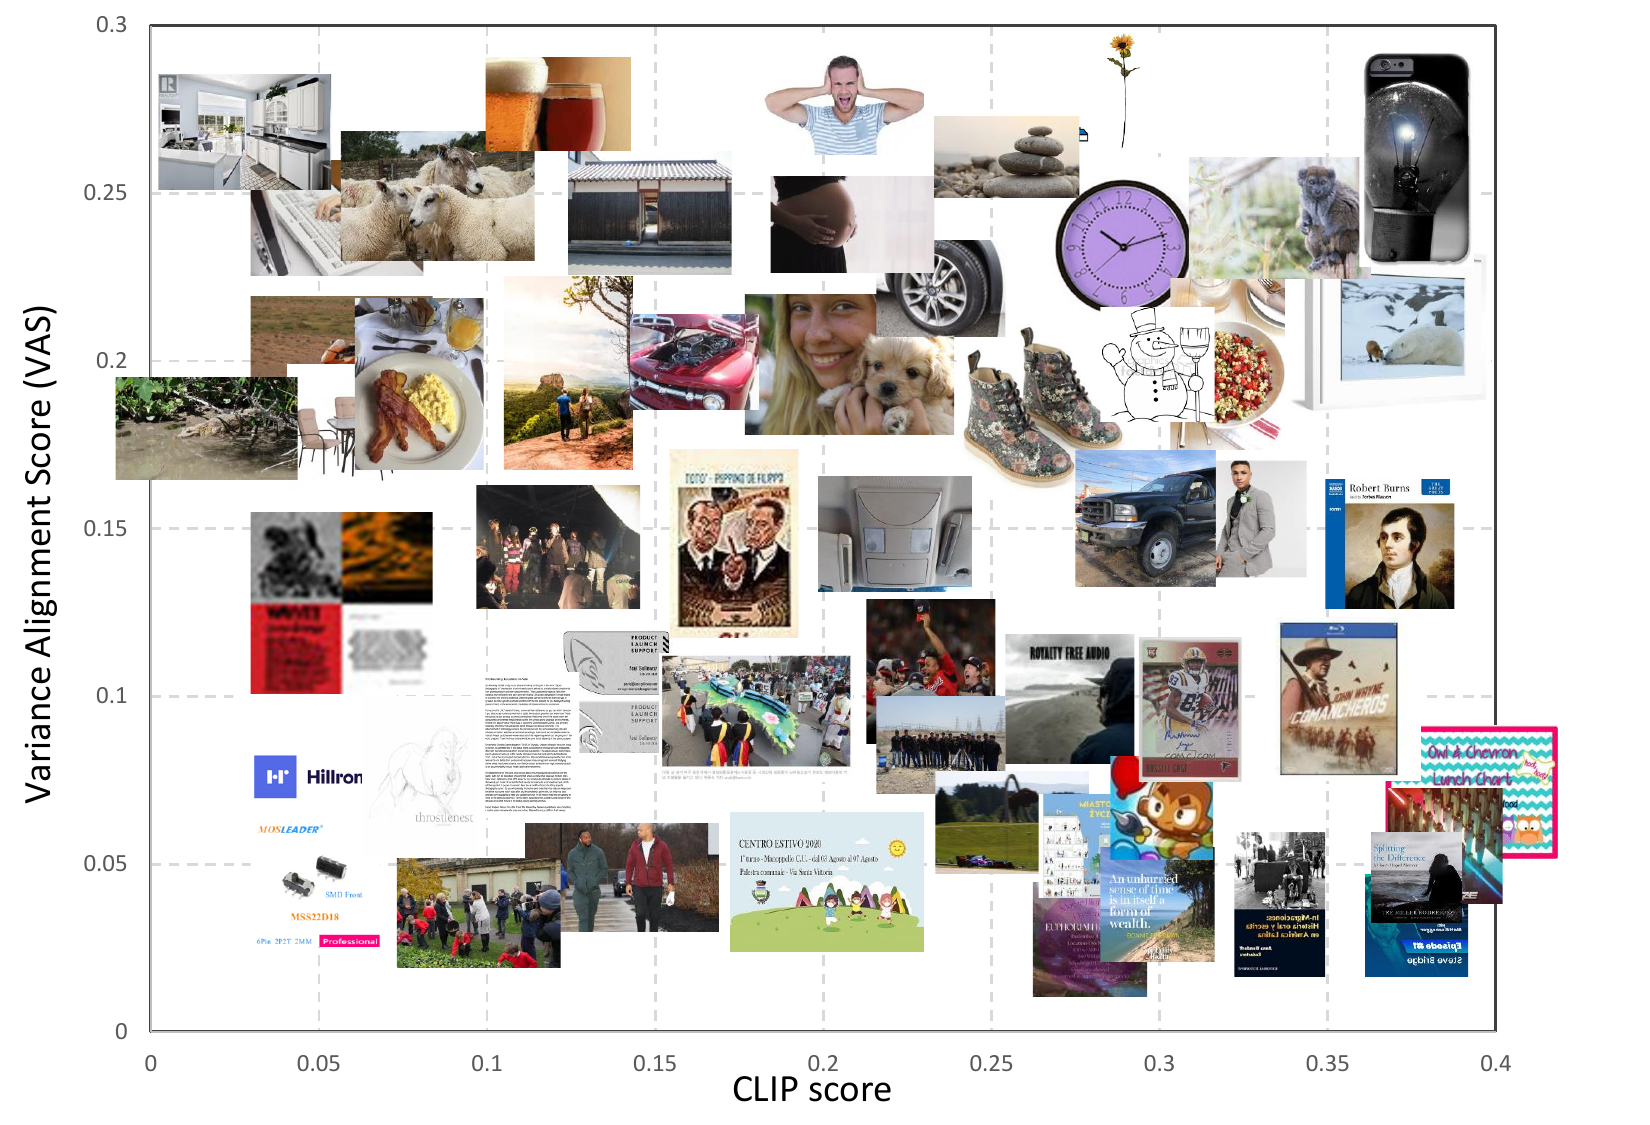}
    \label{fig:visual}
\end{figure*}

\newpage
\begin{figure*}[t]
    \centering
    \caption{Visualization of data pairs with different CLIP scores and VAS in DataComp. Here `img1k\_vas' means VAS(ImageNet-1k) and `self\_vas' denotes VAS(DataComp). We can see that for most of the data, VAS(DataComp) is always similar to VAS(ImageNet-1k).}
    % \vspace{-1em}
    \rotatebox[]{270}{\includegraphics[width=1.2 \textwidth]{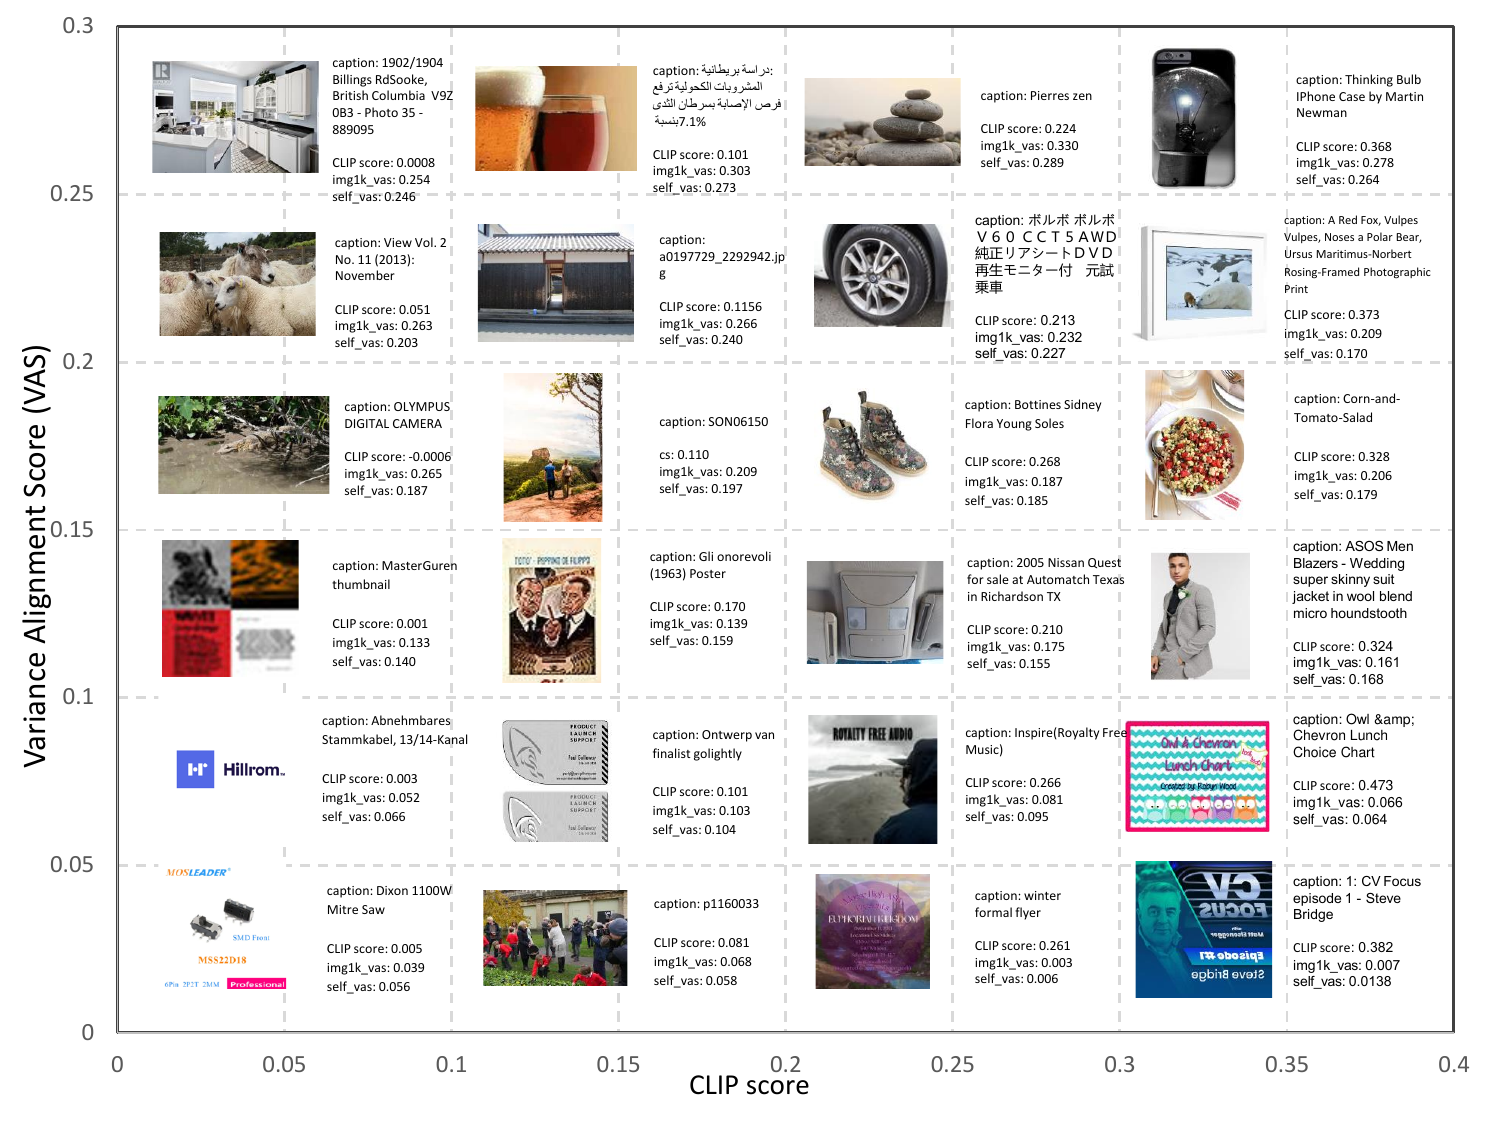}}
    \vspace{-1.0em}
    % \label{fig:vis}
    \label{fig:vis_many}
    \vspace{-0.7em}
\end{figure*}
